# Supplementary material for: Two-mode squeezing and SU(1,1) interferometry with trapped ions
Source: arXiv:2312.10847 source file (2024-07-02)

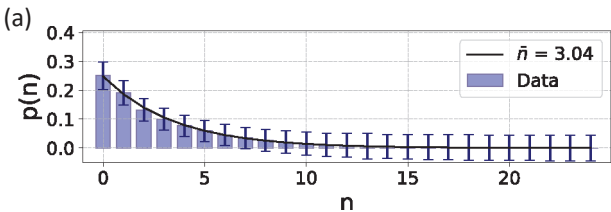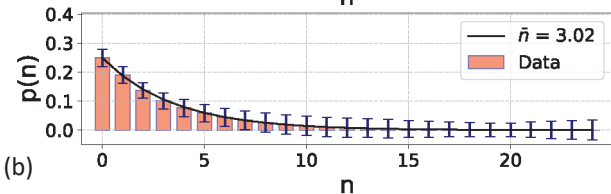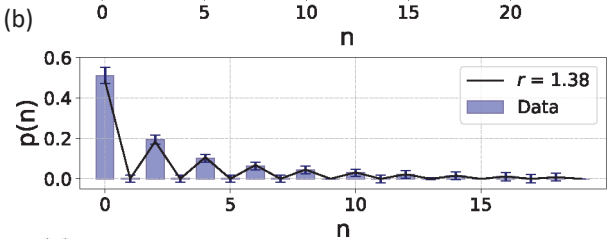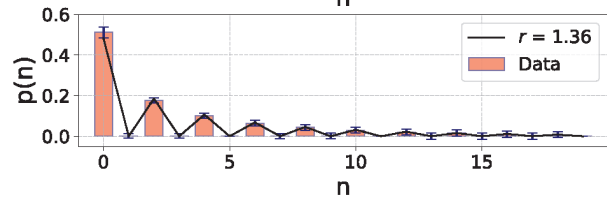

a)

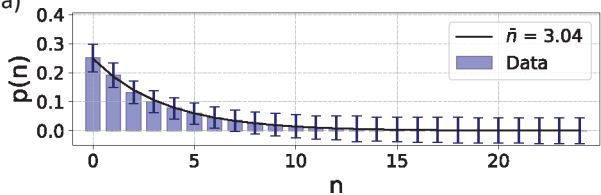

Supplement: Supplementary file 1 [file supp_fig_3_pn_b.pdf]
